# Supplementary material for: Silicene vs. ordered 2D silicide: the atomic and electronic structure of the Si-$(\sqrt{19}\times\sqrt{19})R23.4^{\circ}$/Pt(111) surface reconstruction
Source: arXiv:1402.7275 source file (2014-06-14)
Supplement: Supplementary file 1 [file supp_v7.pdf]

# Silicene vs. 2D ordered silicide: the atomic and electronic structure of the Si-$(\sqrt{19} \times \sqrt{19})R23.4^\circ$/Pt(111)

M. Švec,[1,*] P. Hapala,[1] M. Ondráček,[1] P. Merino,[2] M. Blanco-Rey,[3,4] P. Mutombo,[1] M. Vondráček,[1] Y. Polyak,[1] V. Cháb,[1] J. A. Martín Gago,[5] and P. Jelínek[1,6]

[1]*Institute of Physics AS CR, Cukrovarnická 10, CZ-16200 Prague, Czech Republic*

[2]*Centro de Astrobiología INTA-CSIC, Ctra. de Ajalvir, km.4, ES-28850 Madrid, Spain*

[3]*Dpto. de Física de Materiales UPV/EHU, Apartado 1072, 20018 Donostia-San Sebastián, Spain*

[4]*Donostia International Physics Center, Pº Manuel de Lardizabal 4, 20018 Donostia-San Sebastián, Spain*

[5]*CSIC-ICMM, C/Sor Juana Ines de la Cruz 3, E-28049 Madrid, Spain*

[6]*Graduate School of Engineering, Osaka University 2-1, Yamada-Oka, Suita, Osaka 565-0871, Japan*

(Dated: February 28, 2014)

## PHOTOEMISSION SPECTRA

The photoemission spectra that were crucial for the characterization of the surface were taken at energy 150.15 eV with the incident beam $60^o$ off the normal to the surface and the axis of the detector perpendicular to the surface. The beam energy was monochromated and its diameter was ≈50um, aimed at the center of the sample. The instrument was a Phoibos 150 analyzer with a delay line detector, on the Materials Science Beamline in Trieste. The excitation energy was determined by using a precisely measured Fermi level at the beginning and at the end of these measurements. The reason why this energy was chosen is twofold; first, the sensitivity to Si2p photoelectron doublet rises dramatically and second, the Pt Auger peak at 65 eV (kinetic energy) does not interfere neither with the Si2p nor with the Pt4f doublet. We show the spectra of clean Pt(111) and Si-induced $\sqrt{19}$ reconstruction for the widescan(Fig.1) and Pt4f(Fig.2). On the clean surface, Si (Si2p), O (O1s) and C (C1s) residues were under the detection limit. On the other hand, during the formation of $\sqrt{19}$, C1s peak appeared, but with a negligible intensity. The C1s and O1s only rise to significant levels after prolonged exposure ($>$ 2 hours) to the incident beam and the residual gas in the chamber. The Pt4f and the Auger peak at 85 eV all exhibit an intensity drop induced by the formation of $\sqrt{19}$. Pt4f has a significant change in the shape, when the surface-related peak (marked as S2 in Fig.2) splits in two components (S2' and S2"), while the S1 and S3 components attributed to the remain almost unchanged. Evaluation of the coverage using the Si2p and Pt4f total areas gives a concentration of 6 Si atoms per unit cell. We assume the mean escape depth of the photoelectrons correspond to 4 atomic layers of the Pt(111). Moreover, the ratio of the Pt4f surface component in Fig.1 is ≈0.55. In the best-fit model, the ratio of surface Pt atoms that have 3 neighbours to the rest of them is 8:7(=1.14). All spectra were normalized to the beam intensity changes during time.

## DYNAMIC ATOMIC FORCE MICROSCOPY

The combined scanning tunneling microscopy and dynamic atomic force microscopy (STM/dAFM) images were taken using a custom-built and calibrated tuning-fork sensor [1] with a resonance frequency of 47520 Hz with a stiffness 3400 $N.m^{-1}$. The Fig.3 shows a simultaneous measurement of STM and dAFM. At the first glance, the protrusions in the

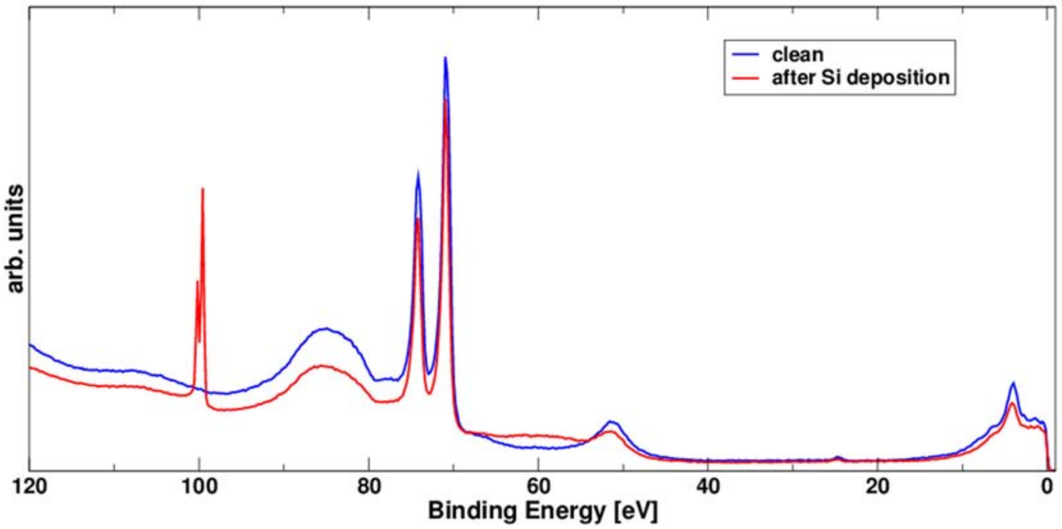


FIG. 1. The photoemission widescan spectra at 150 eV photon energy. The principal Pt4f doublet at 71 eV is dominant, as well as the Auger peak at 85 eV (corresponding to 65 eV kinetic energy). After formation of $\sqrt{19}$, Si2p appears around 100 eV.

STM image that are ascribed to the top Pt atoms of the final model are also brighter in the $\Delta$f map. These protrusions are exerting a repulsive force on the probe. This is a clear evidence that these atoms are protruding out from the surface plane.

## GRAPHENE ON THE $\sqrt{19}$

Accidentally, we grew graphene layer simultaneously with the $\sqrt{19}$ structure, see the Fig.4. This sample was not cleaned by the standard cycles of $Ar^+$ bombardment and annealing, such that contamination could accumulate on its surface during several days before this experiment. Afterward, the $\sqrt{19}$ structure was formed by the standard recipe. Surprisingly, not only the $\sqrt{19}$ was found, but also a full overlayer of graphene, manifested by honeycomb pattern superimposed onto the $\sqrt{19}$. On the parts of Pt surface that remained clean, the typical Moiré modulation appears. The lattice distances of graphene determined with respect to the $\sqrt{19}$ match well its natural value, 2.46 Å. The formation of graphene was most likely caused by presence of the CO molecules or other volatile carbon-containing compounds that form the residual atmosphere of the experimental STM/AFM chamber.

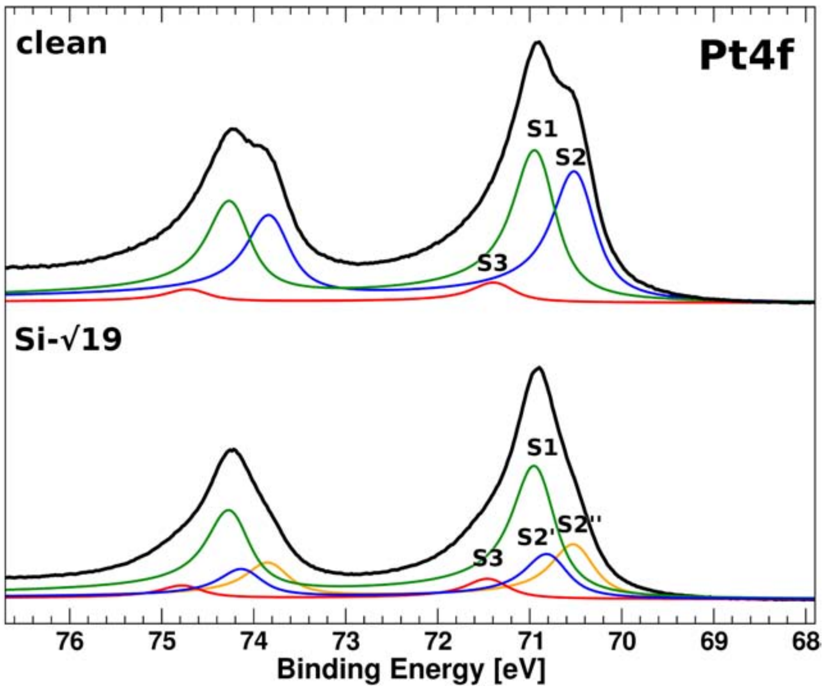


FIG. 2. The photoemission spectra of Pt4f doublet (at 150 eV photon energy) fitted by three components for the clean surface and four components for the Si-induced $\sqrt{19}$ superstructure. It shows that the surface-related state at lower binding energy splits upon the formation of $\sqrt{19}$ and the overall intensity decreases. The inset shows the Si2p before and after the deposition of 0.3ML Si with sample at 650$^o$C.

**NANOESCA**

The used instrument NanoESCA is a photoemission spectrometer based on PEEM column and a double hemispherical imaging energy filter. The aberrations of the first hemispherical analyzer are compensated with the help of a second hemisphere, such that the inner electron trajectories in the first hemisphere become the outer trajectories in the second hemisphere. The monochromatized AlK$\alpha$1,2 X-ray source can be focused to illuminate a spot of the size between 10-100 $\mu$m. A voltage 15 kV is applied to accelerate electrons emitted from a sample and entering the column. The overall resolution of the spectroscopic system is 0.3-0.4 eV. An important design concept of this instrument is the ability to switch between spatial and momentum imaging. Changing the number of lenses in PEEM (from 3 to 2) we performed the k-space mapping in the combination with the HeI discharge lamp. It allows to image electron states at a position chosen in the real space imaging mode. The arrangement of the

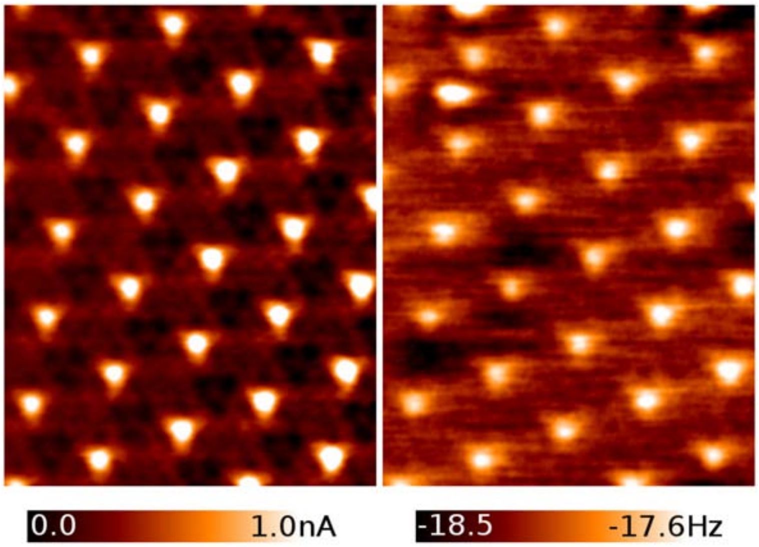


FIG. 3. Simultaneous STM (left) and AFM (right), taken on the $\sqrt{19}$. The image is taken with 200 pm amplitude, -18Hz $\Delta$f setpoint and -25 mV bias. The regularly spaced bright locations in $\Delta$f correspond to the top Pt atoms, that protrude slightly of the surface.

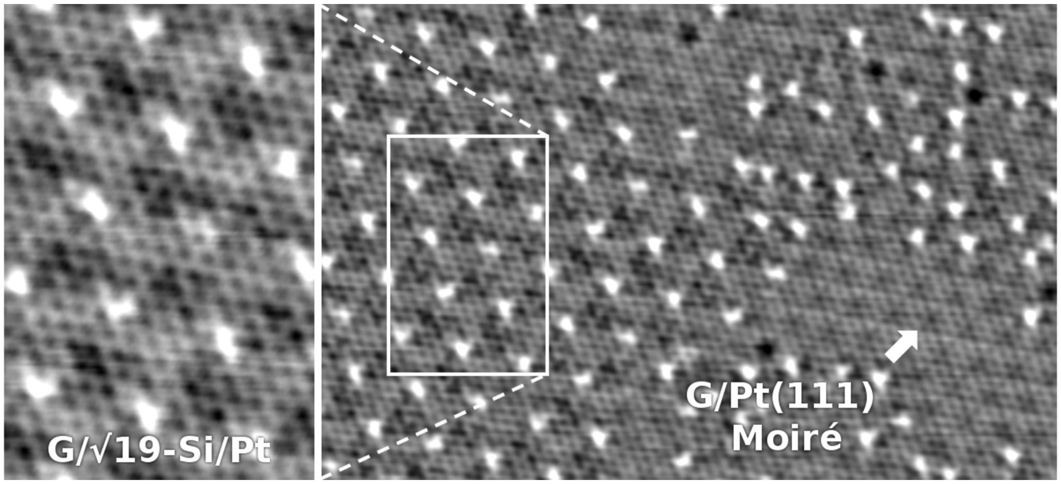


FIG. 4. Graphene grown on the Si-$\sqrt{19}$/Pt(111) surface. The zoomed area($3.1 \times 4.7$ nm$^2$) was taken separately with the STM at higher resolution. Measurement parameters were 100mV bias voltage, 1 nA tunneling current feedback. The image size: $14\times9$ nm$^2$.

lenses and apertures in the column transmit a large angular range (i.e. the k-space usually covers the first Brillouin zone or more). The energy resolution of the energy cuts is 0.1 eV. The pressure in the UHV chamber did not exceed $5 \times 10^{-10}$ mbar.

## TOTAL ENERGY CALCULATIONS

### Si/Pt(111)

There were in total more than ten candidate models of the $\sqrt{19}$ unit cell structure. All of them were based on a 4-layer slab of the $\sqrt{19}$ Pt(111) unit cell. Afterward, they have been modified around the centers of the observed bright and dark triangular protrusions. Considering the first subsurface layer and its stacking with the top layer, these two positions had to be treated as nonequivalent. Pt-Si tetrahedrons have been substituted for three Pt atoms at each of these two positions, as illustrated by Fig. 5. Using this method, nine basic models were created and optimized using the FIREBALL code. A concrete example of the relaxation process for the best-fit model is shown in Fig. 8. We also put on trial some less probable substitutions, which however resulted in solutions that had very unfavorable energy.

The geometry optimization and total energy calculations were first done with a tight-binding *ab initio* code FIREBALL [2, 3]. FIREBALL uses an optimized spatially-confined pseudo-atomic orbital basis set. In our case, an *sp* basis set was used for the Si atoms and a *spd* basis set for the Pt atoms. The cutoff radii of the pseudo-atomic basis functions were as follows: $R(\mathrm{Si}, s) = 4.8$ a.u., $R(\mathrm{Si}, p) = 5.48$ a.u., $R(\mathrm{Pt}, s) = 4.2$ a.u., $R(\mathrm{Pt}, p) = 4.6$ a.u., and $R(\mathrm{Pt}, d) = 5.4$ a.u. Local density approximation is assumed for the exchange correlation functional. The first surface Brillouin zone of the $\sqrt{19}$ unit cell was sampled by $6 \times 6$ $k$-points. The bottom Pt atomic layer of the 4-layer slab was kept fixed during the geometry optimization while all other atoms were allowed to relax freely into their equilibrium positions. The criterion for terminating the relaxation was that maximal forces on free atoms had to be below 0.05 eV/Å and the change of total energy between subsequent iterations had to be smaller than $10^{-4}$ eV per unit cell.

For the two most stable models (A and D) and a "silicene" model (a monoatomic layer of Si on the Pt substrate in a honeycomb arrangement, 18 Si atoms per $\sqrt{19}$ surface cell), the calculation was repeated with the pseudopotential code VASP [4–7], see Ref. [8, 9] for the type of ultrasoft pseudopotentials implemented in VASP. The plane wave cutoff was set to 300 eV. The PW91 generalized gradient approximation [10, 11] was used as the exchange-correlation functional. The first surface Brillouin zone of the $\sqrt{19}$ unit cell was

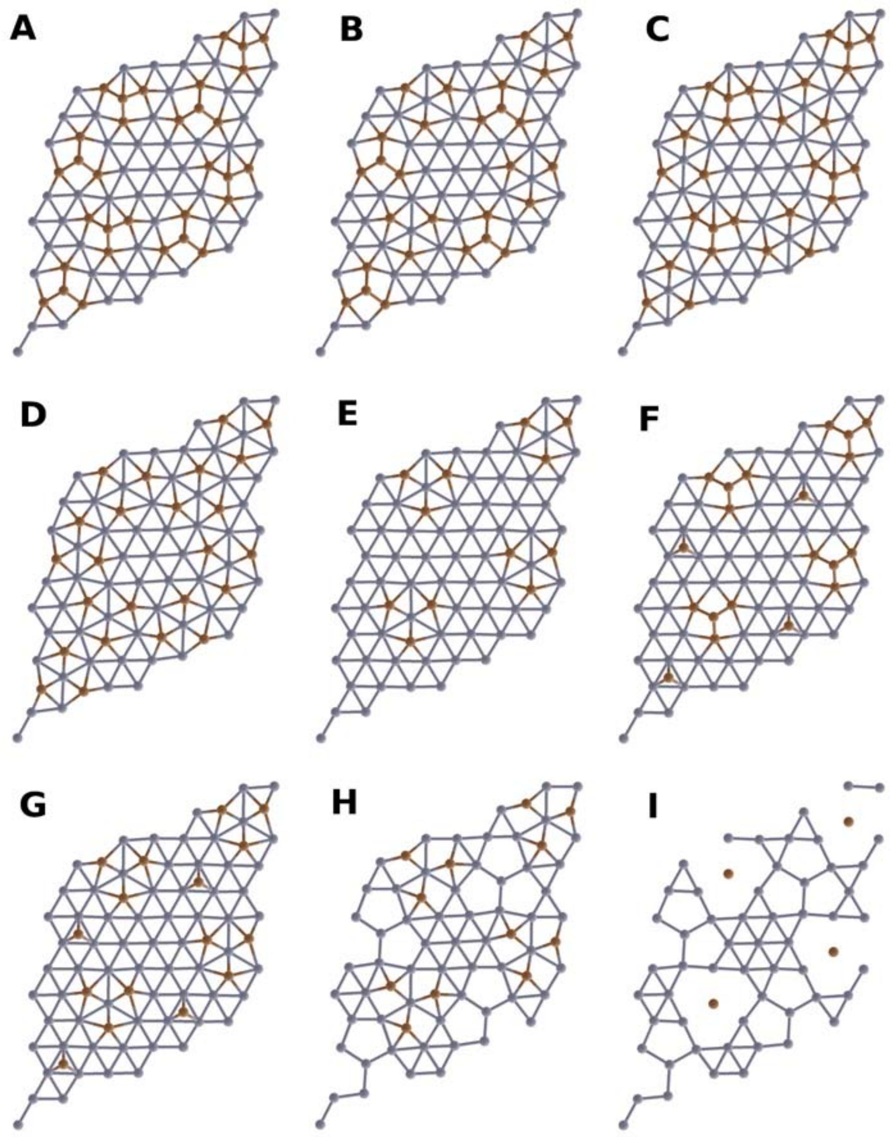


FIG. 5. The overview of the models used for the calculation; all of them were created by replacing one or two triplets of surface Pt atoms by a Si/Si-Pt tetrahedron or an atom. The shown models are only the topmost layer of the slab used for the calculation, 2× repeated in both surface-lattice directions. Color code: Si atoms yellow, Pt atoms gray.

again sampled by $6 \times 6$ $k$-points. The relaxation was terminated when forces on all free atoms had all their Cartesian coordinates below 0.001 eV/Å. This criterion corresponded roughly to the precision of $10^{-6}$ eV per unit cell.

We had to establish a criterion for comparing the stability of models with different numbers of atoms in the unit cell. We use the excess of surface energy per $1 \times 1$ surface unit

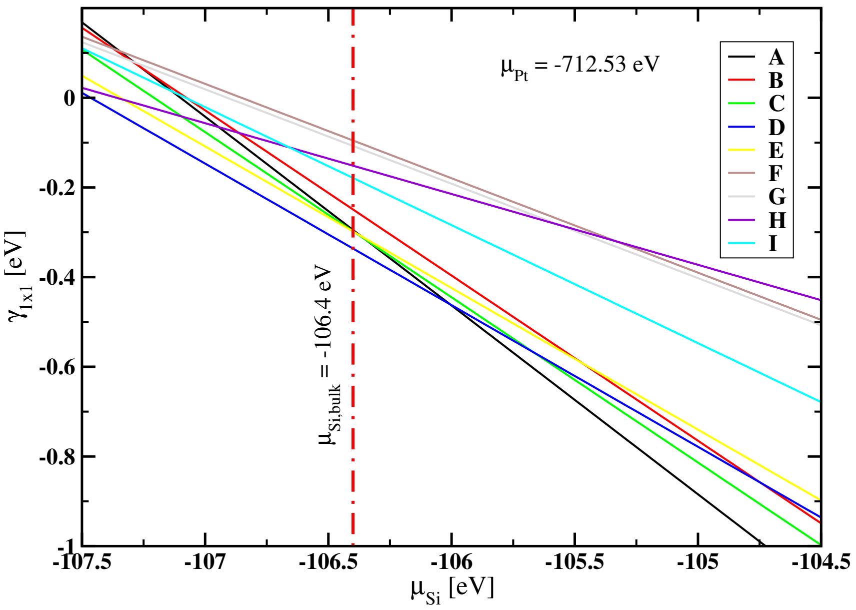


FIG. 6. Comparison of different models in terms of their stability. We relate the stability of different structures to the excess surface energy $\gamma_{1\times1}$, as defined in the text. Results obtained with the FIREBALL code are shown here. The red dash-dotted vertical line denotes the value of Si chemical potential $\mu_{\rm Si}$ that corresponds to the energy of Si atom in the bulk of silicon crystal.

cell in comparison to the surface energy of a clean Pt(111) surface. We define this excess surface energy as

$$\gamma_{1\times1} = (E_{\rm tot} - E_{\rm Pt(111)} - N_{\rm Si}\times\mu_{\rm Si} - N_{\rm Pt}\times\mu_{\rm Pt})/19,$$

where $E_{\rm tot}$ is the total energy calculated for the given Si/Pt(111) model in a $\sqrt{19}$ unit cell, $N_{\rm Si}$ is the number of Si atoms in the model, $N_{\rm Pt}$ is the excess of Pt atoms in the model compared to the $\sqrt{19}$ unit cell of a clean Pt(111) surface, $\mu_{\rm Si}$ and $\mu_{\rm Pt}$ are the respective chemical potentials of Si and Pt atoms, and $E_{\rm Pt(111)}$ is the total energy calculated for a slab that represented a clean Pt(111), also calculated in the $\sqrt{19}$ unit cell. The results are presented in Figs. 7 and 6. The excess surface energy $\gamma_{1\times1}$ is plotted there as a function of the Si chemical potential, $\mu_{\rm Si}$. The energy of Pt atom calculated for bulk platinum was substituted for $\mu_{\rm Pt}$. Because the Pt substrate can serve as a reservoir of platinum atoms, this should be a reasonable assumption. Chemical potentials of Si just below the value estimated as the energy of Si atoms in the bulk silicon crystal can be expected to

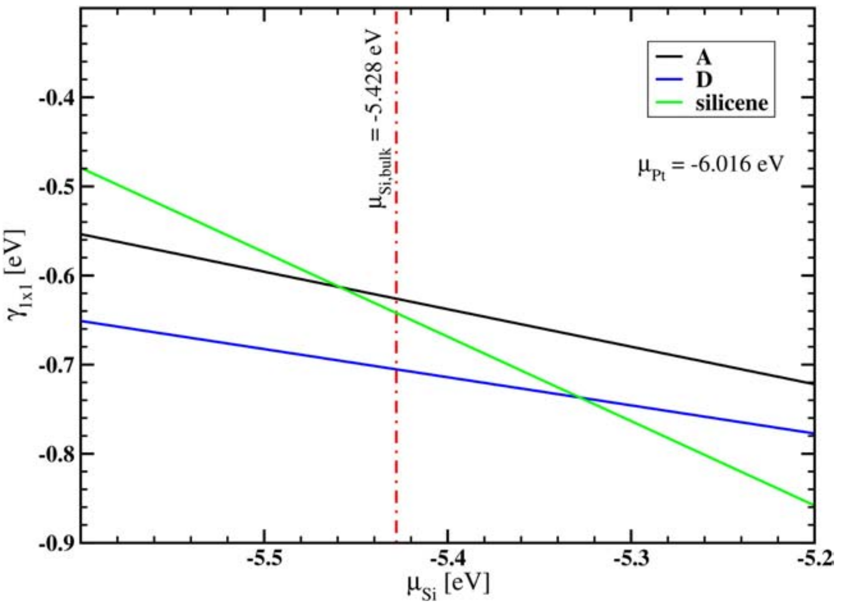


FIG. 7. Comparison of three selected models in terms of their stability. Results obtained with the VASP code are shown here. The red dash-dotted vertical line denotes $\mu_{\rm Si}$ that corresponds to the energy of Si atom in the bulk of silicon crystal.

characterize the availability of Si on the surface, where about one monoatomic layer of Si has been deposited. Note that the absolute values of the calculated total energies depend on the pseudopotentials used in the calculation and have no physical meaning; only quantities expressed as changes or differences of total energies are physically relevant.

In Fig. 7, stability of the two most energetically favorable models (called A and D previously), and the silicene model are evaluated depending on the chemical potential. In the vicinity of the realistic chemical potential value, the most energetically favorable model seems to be the model A, however silicene is only slightly worse. On the other hand, it should be reminded, that at this stage the relaxed honeycomb structure of Si is strongly hybridized with the substrate; therefore the properties associated with $\pi$-bonded materials (as graphene) can not be expected.

**Si/Ir(111)**

We also checked whether the $\sqrt{7} \times \sqrt{7}$ structure (abbreviated as $\sqrt{7}$ in the following) reported for Si on Ir(111) in [12] could be in fact explained by a structural model similar to the one we propose for Si/Pt(111). We constructed such a model by replacing three

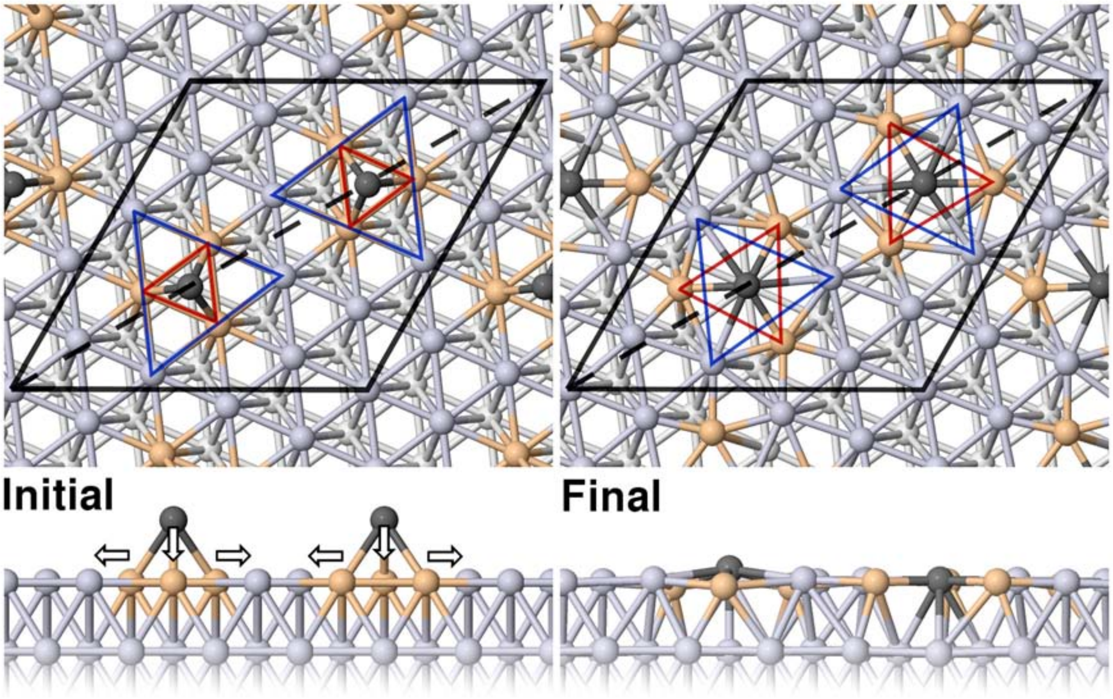


FIG. 8. Detailed view of the most stable structural model (Model D from Fig. 5; top and side views). The black rhombus delimits one $\sqrt{19}$ surface unit cell. On the left: The initial geometry of the D model (before optimization). In each half unit cell, three neighboring Pt atoms have been replaced by Si atoms to form the triangular basis of a Pt-Si tetrahedron. A Pt adatom (dark gray) forms the top vertex of the tetrahedron. On the right: The D model after geometry optimization. The Si triangles (red) expand as the Si atoms move away from the triangle's center (compare also the red Si triangles with the blue triangles formed by the nearest Pt atoms). The Pt adatoms have moved down so much that one of them virtually aligns with the surface atomic layer and the other one remains only about 0.4 Å above the surface layer.

Ir atoms around an fcc-type hollow site by Si atoms and adding one Ir adatom on top of the fcc hollow site to form an $Si_3Ir$ tetrahedron. We will refer to this model as the $Si_3Ir$ model. After relaxation, the Ir adatom moved down and became part of the surface layer. We compare the $Si_3Ir$ model with another model, which represents a silicine structure. This "silicene" model was essentially the same as the one considered in Ref. [12]: a honeycomb structure consisting of 6 Si atoms in the $\sqrt{7}$ unit cell placed on top of an unreconstructed Ir(111) surface. One of the six Si atoms was placed directly on an Ir atom and another one in a hcp hollow site of the iridium surface.

The geometry optimization and total energy calculations were performed using the VASP code. We used the same parameters in the calculations with VASP for the Si/Ir(111) models as we did for the Si/Pt(111) models. The first surface Brillouin zone of the smaller $\sqrt{7}$ unit cell (compared to the $\sqrt{19}$ cell) was sampled by $9 \times 9$ $k$-points.

In order to compare the total energies calculated for the different structural models of Si/Ir(111), we adapted our formula for the excess surface energy per $1 \times 1$ surface unit cell to the case of the $\sqrt{7}$ cell and the Ir(111) surface:

$$\gamma_{1\times1} = (E_{\text{tot}} - E_{\text{Ir}(111)} - N_{\text{Si}} \times \mu_{\text{Si}} - N_{\text{Ir}} \times \mu_{\text{Ir}})/7.$$

Here again, $E_{\text{tot}}$ is the total energy calculated for the given Si/Ir(111) model in a $\sqrt{7}$ unit cell, $N_{\text{Si}}$ is the number of Si atoms in the model, $N_{\text{Ir}}$ is the excess of Ir atoms in the model compared to the $\sqrt{7}$ unit cell of a clean Ir(111) surface, $\mu_{\text{Si}}$ and $\mu_{\text{Ir}}$ are the respective chemical potentials of Si and Ir atoms, and $E_{\text{Ir}(111)}$ is the total energy calculated for a clean Ir(111) surface, also calculated in the $\sqrt{7}$ unit cell. The results are presented in Fig. 9. The excess surface energy $\gamma_{1\times1}$ is a function of the Si chemical potential, $\mu_{\text{Si}}$. The energy of Ir atom calculated for bulk iridium was substituted for $\mu_{\text{Ir}}$.

## STM IMAGE SIMULATIONS

The optimized geometry from VASP was used in simulations of STM images for the proposed structures. The model of the STM tip was a four-sided tungsten pyramid derived from the W(100) surface structure. The STM simulations were carried out using the STM code, which uses Green's function formalism to evaluate the tunneling current [13]. The Green's functions were calculated from a local basis set Hamiltonian obtained from the Fireball code using the optimized atomic structures of a given model. Constant height images corresponding to a tip height of 4 Å over the surface and to a surface bias of +20 mV were computed. The Fireball basis set specified in the previous section was used for Si and Pt atoms in deriving the density of states projected on orbitals of the surface atoms. In order to calculate the density of states projected on orbitals of a tungsten atom on the tip, a *spd* basis set with the following cutoff radii was used: $R(\text{W}, s) = 4.7$ a.u., $R(\text{W}, p) = 5.2$ a.u., and $R(\text{W}, d) = 4.7$ a.u. The projected densities, which subsequently entered the current calculation. Pseudo-atomic functions with an enlarged cutoff radius $R = 15$ a.u. were

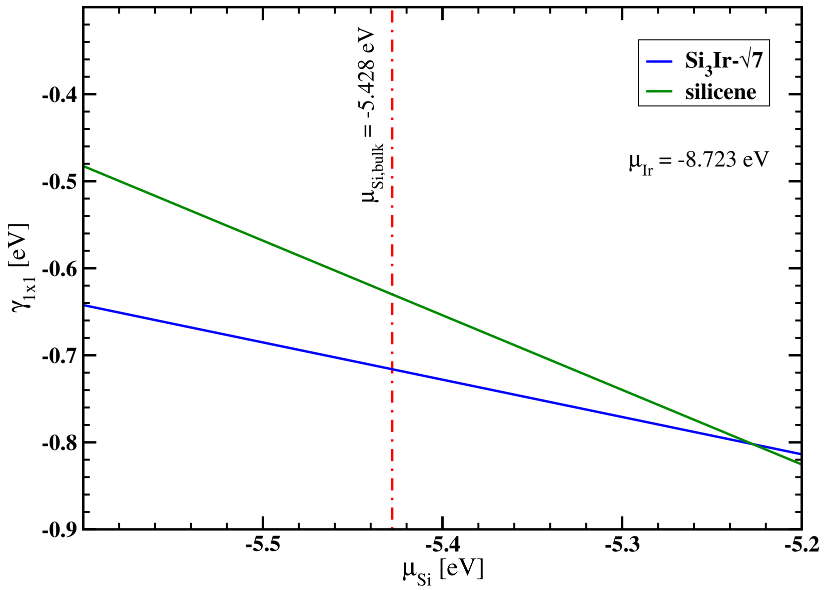


FIG. 9. Comparison of two Si/Ir(111) models in terms of their stability. Both the $Si_3Ir$ and the silicene model are described in the text, as well as the formula that gives the dependence of excess surface energy $\gamma_{1\times1}$ on silicon chemical potential $\mu_{\rm Si}$. The red dash-dotted vertical line denotes $\mu_{\rm Si}$, which corresponds to the energy of Si atom in the bulk of silicon crystal.

employed to derive the interatomic hopping (tunneling) probabilities between the surface atoms and an atom on the tip. Only the outermost tip atom, the Si atoms (and Pt adatoms) on the surface, and atoms of the topmost surface layer and one subsurface Pt layer were considered for tunneling. The first surface Brillouin zone was sampled by $4 \times 4$ $k$-points for the purpose of STM simulations.

## LEED-IV - EXPERIMENT AND CALCULATIONS

The LEED-IV experiment was performed on a standard LEED instrument. The azimuthal and polar angles of the sample adjustment was done using the equivalent diffraction spot variations, in order to ensure the sample was perpendicular to the incident electron beam. The LEED-IV curves were created using a series of video images taken with a high-sensitivity monochrome CCD camera in a focal distance from the fluorescent screen. A custom program was used to control the electron energy and to average the images for every

energy step. Each image is thus an average of 64 video frames taken at 1.21A filament ($LaB_6$) current, 4 kV screen voltage. The resolution of the images was 768×576 pixels with a depth of 8 bits. Intensity maximum of the LEED pattern was kept below the saturation level of the CCD in the whole range of measured energies. Sets of images were taken for the clean and the $\sqrt{19}$ structure. The data was evaluated using another custom program written in Interactive Data Language (IDL). Every spot has been evaluated separately to obtain the intensity profile depending on the energy. Typically, we were able to measure IV curves for three equivalent fractional spots, which allowed to evaluate their mutual Pendry R-factors [14] and trim their energy ranges to keep these R-factors below 0.3. In the final step, curves for each spot have been averaged and used as the input for the calculation.

Theoretical LEED intensities as a function of energy, or IV curves, were obtained from full-dynamical calculations, i.e. taking full account of the multiple scattering events undergone by scattered electrons. Pendry's reliability factor, $R_P$, was used to quantify the agreement between the experimental and theoretical IV curves [14]. Automated searches were performed in order to optimize the structure, this is, the objective is to find the structure that yields the smallest possible $R_P$. The code CLEED [15] was used for these purposes.

Electron scattering by each ion-core in the surface is well described by a central potential, and it is thus characterized by a set of phase shifts. The potentials were obtained from first-principles calculations within the Density Functional Theory (DFT) with the generalized gradient formulation of the exchange and correlation potential [16] for bulk Si and Pt. The code FLEUR was used, that is based in the all-electron Full-Potential Linearized Augmented Plane Wave (FLAPW) formalism [17, 18]. Within this formalism, the space is divided into non-overlapping regions associated to the ion cores, called "muffin-tins" (MT). The basis set for the electronic wave-functions consists of partial waves inside the MTs and plane waves in the interstitial region. The spherical component of the potential inside the MTs was taken to generate the phase shifts up to an quantum angular momentum number $l_{max} = 7$ by solving the corresponding one-electron radial Schrodinger equation. The wavefunction plane wave basis for the interstitial region was constructed with energy cut-offs 300 eV and 318 eV for Si and Pt, respectively, and special k-point meshes $12 \times 12 \times 12$ and $9 \times 9 \times 9$ for Si and Pt, respectively [19]. The MT radii used in this work are 2.20 and 2.55 a.u. for Si and Pt, respectively.

In the model structures the Pt substrate lattice constant was set to match the experimen-

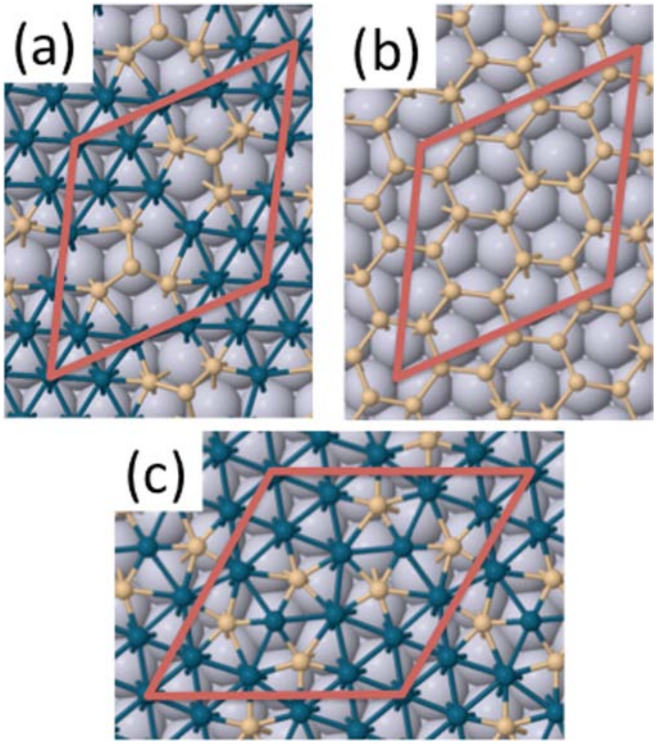


FIG. 10. Si/Pt(111) models considered in the LEED-IV analysis: (a) model A, (b) silicene and (c) model D. Substrate Pt atoms are depicted as large gray balls. Reconstructed overlayer Pt atoms are shown as smaller blue balls. Si atoms are shown in yellow. The $(\sqrt{19} \times \sqrt{19})$ reconstruction unit cell is plotted in red.

tal Pt-Pt distance, 2.774 Å [20]. Only the $z$ coordinates of the SiPt reconstructed overlayer were used in the optimization process, while the lateral fractional coordinates were kept fixed at their DFT positions. LEED-IV curves for the two lower energy models resulting from the DFT calculations with VASP [7], were calculated (see Figure 10). This procedure allows us to rule out two of them, namely the silicene and the A models, as they result in R-factor values of 0.70 and 0.75, respectively. The trimer model turns out to be the best structure, which yields $R_{P,min} = 0.335$ after optimization. The corresponding 21 structural parameters can be found in Table I. The error bars in $z$ were calculating taking into account that any model that yields $R_P < R_{P,min}(1 + RR)$ is statistically acceptable [14]. Here, $RR = \sqrt{8V_{0i}/\Delta E}$ and $\Delta E = 1004\,\mathrm{eV}$ is the total energy extent of the experimental IV database. The best fit LEED-IV curves are shown in Figure 11. The used beams, corresponding to both integer and fractional order LEED spots, are sketched in Figure 12. In the optimized trimer structure, the buckling of the overlayer is much stronger than the one

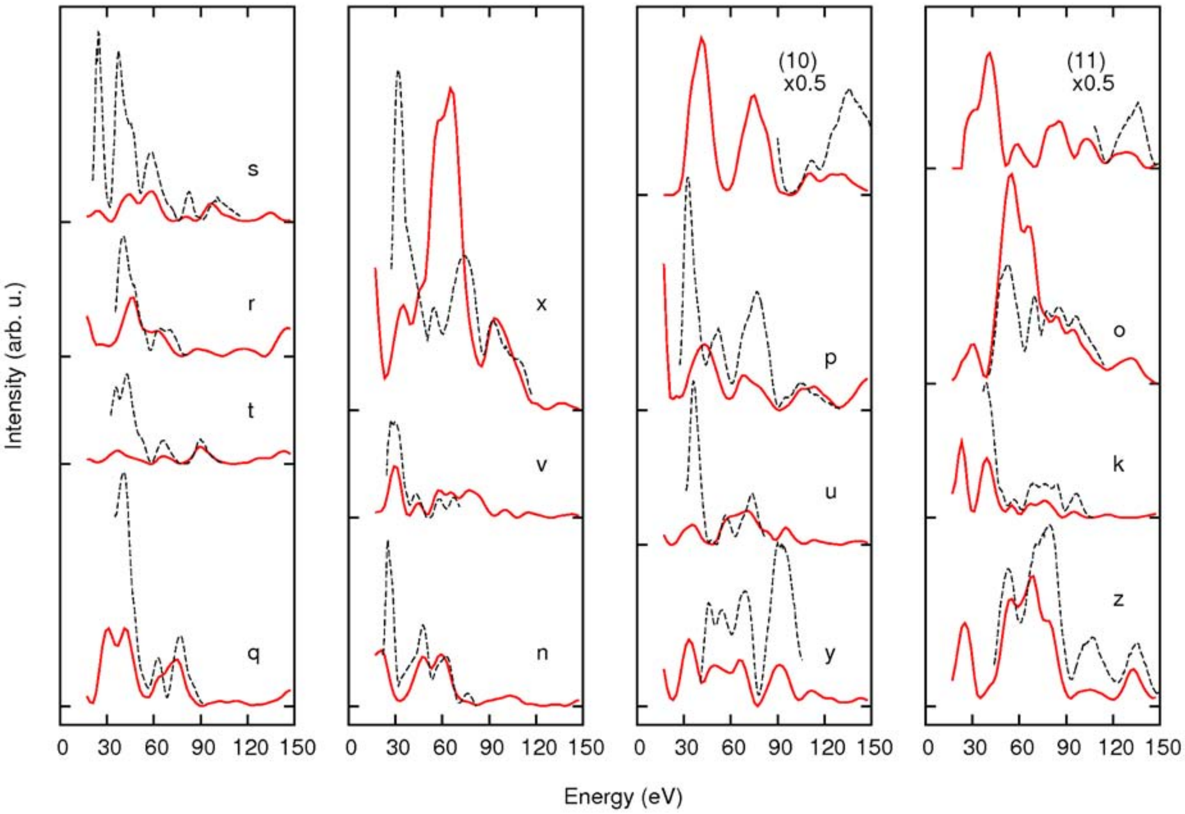


FIG. 11. LEED-IV curves for the best fit trimer structure. Solid (dashed) line is the theoretical (experimental) result. The beam labels correspond to the LEED spots as sketched in Figure 12.

obtained in the DFT calculation with VASP.

However, the displacements in $z$ associated to the buckling are of the same order as the error bars in the corresponding coordinates. Thus, the present LEED-IV analysis cannot fully resolve the fine details of the structure buckling. The main structural feature found by VASP, namely the Pt that is pushed $\gtrsim 0.3\,\text{Å}$ out of the surface (labeled as Pt1 in the table), is kept after the LEED-IV analysis.

Other non-structural parameters in the search are $V_{0r} = -10.5$ and $V_{0i} = 4\,\text{eV}$ for the real and imaginary parts of the inner potential, respectively. Vibrational movement of the surface atoms is accounted for by isotropic Debye-Waller factors in the ion-core scattering factors. A root mean square vibrational amplitude value 0.09 Å has been set for the substrate Pt atoms, which corresponds to a Debye temperature of 230 K. Optimized values for the overlayer atoms are 0.14 and 0.11 Å for Si and Pt, respectively. Thus, a total of 23 parameters have been

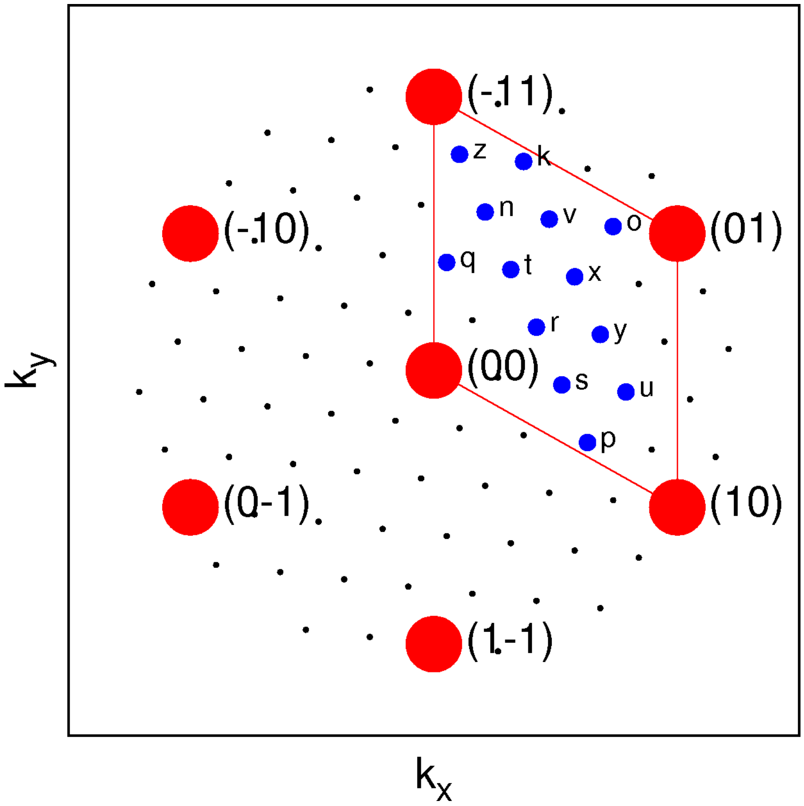


FIG. 12. LEED-IV spots. Sketch of the reciprocal lattice. The large red (small black) dots correspond to integer (fractional) order LEED spots in the experiment. The medium-sized blue dots represent the beams used in the structure optimization.

considered in the present search.

## PROJECTION OF CALCULATED BAND STRUCTURE FOR COMPARISON BETWEEN DIFFERENT RECIPROCAL UNIT CELLS AND ARPES

Here we describe a projection method that allows us to map out the electronic band structure obtained from a typical total energy calculations (such as DFT) beyond the first Brillouin zone (1. BZ). This is necessary for comparison of the band structures between different surface reconstructions with different unit cells, as well as for comparison with ARPES experiment.

Typical total energy calculations of a particular reconstruction (e.g. the $\sqrt{19}$ ) are performed using a set of $k$-vectors spawned from the 1. BZ of the corresponding supercell. The supercell is typically much larger and contains more atoms than the unit cell of the

TABLE I. $(x, y, z)$ coordinates in Å of trimer structure overlayer atoms after LEED-IV optimization.

| | $x$ | $y$ | $z$ |
|---|---|---|---|
| Si1 | 2.94 | -2.54 | 2.20 (± 0.08) |
| Si2 | 4.65 | -6.08 | 2.24 (± 0.10) |
| Si3 | 0.72 | -5.79 | 2.28 (± 0.10) |
| Si4 | 9.06 | 1.75 | 2.35 (± 0.12) |
| Si5 | 5.05 | 2.17 | 2.30 (± 0.08) |
| Si6 | 6.69 | -1.51 | 2.32 (± 0.10) |
| Pt1 | 2.77 | -4.80 | 2.70 (-0.10/+0.14) |
| Pt2 | 6.94 | 0.80 | 2.37 (-0.12/+0.16) |
| Pt3 | 1.50 | -0.74 | 2.41 (-0.10/+0.14) |
| Pt4 | 7.00 | 3.70 | 2.44 (-0.16/+0.08) |
| Pt5 | 9.41 | -0.70 | 2.35 (± 0.16) |
| Pt6 | -0.11 | -7.94 | 2.24 (± 0.16) |
| Pt7 | 2.77 | 1.73 | 2.35 (-0.20/+0.12) |
| Pt8 | 4.40 | -0.59 | 2.33 (-0.16/+0.10) |
| Pt9 | 5.27 | -3.42 | 2.43 (-0.08/+0.12) |
| Pt10 | 6.94 | -5.73 | 2.29 (± 0.12) |
| Pt11 | 9.82 | 3.94 | 2.32 (-0.20/+0.24) |
| Pt12 | 0.33 | -3.33 | 2.37 (-0.16/+0.12) |
| Pt13 | 2.72 | -7.66 | 2.43 (-0.16/+0.12) |
| Pt14 | 8.21 | -3.27 | 2.19 (± 0.12) |
| Pt15 | 0.00 | 1.60 | 2.26 (-0.08/+0.20) |

unreconstructed surface (e.g. the Pt(111)-(1 × 1)). This means that the computed band structure contains more bands than the original band structure of (1 × 1) unit cell (i.e. the bands are folded into the smaller 1. BZ ).

On the other hand, the electronic band structure measured in an ARPES experiment

does not naturally depend on the supercell choice, so it is not *folded* into any particular 1. BZ. In order to obtain the *unfolded* band structure we need to compute the projection of our computed Bloch states $\psi_{i,k}(r)$ onto an arbitrary plane wave $e^{-ik.r}$, which will filter out all the bands folded from different reciprocal unit cells.

The eigenfunction $\psi_{i,k}(r)$ of $i$-th band of $k$-vector can be expressed as a linear combination of atomic-like orbitals $\chi_\nu(r)$:

$$\psi_{i,k}(r) = \sum_\nu e^{-ik.R_\nu} a^i_\nu(k)\chi_\nu(r), \tag{1}$$

where $R_\nu$ represents a position of the atom, where the localized basis $\chi_\nu(r)$ is centered and $i$ stands for index of band. The coefficients $a^i_\nu(k)$ are obtained diagonalizing Kohn-Sham Hamiltonian $H^{KS}$ written in the local orbital formalism, which is expressed as follows:

$$\sum_\mu [H^{KS}_{\mu,\nu}(k) - \epsilon_i(k)S_{\mu,\nu}(k)]a^i_\nu(k) = 0, \tag{2}$$

where $\epsilon_i$ represents $i$-th eigenvalue and $S_{\mu,\nu}$ the overlap matrix at a given $k$-vector. The matrices $H^{KS}_{\mu,\nu}$, $S_{\mu,\nu}$ are defined as:

$$H^{KS}_{\mu,\nu}(k) = \int dr e^{ik.(R_\nu - R_\mu)}\chi_\mu(r)\hat{H}\chi_\nu(r), \tag{3}$$

$$S_{\mu,\nu}(k) = \int dr e^{ik.(R_\nu - R_\mu)}\chi_\mu(r)\chi_\nu(r). \tag{4}$$

Usually, in DFT calculations the $k$-vectors are restricted to the first Brillouin zone. On the other hand, the band structure measured by ARPES is in principle the projection $P^i_k$ of Bloch states $\psi_{i,k}(r)$ onto a plane wave $e^{-ik.r}$ which represents the lateral component of incident ( X-ray, UV ) light waves. The $k$-vector of light is not constrained in the first BZ of the surface reconstruction and the obtained band structure is *unfolded*. Therefore, we solve Eq. 2 at a set of $k$-vectors, which can be also located outside of the first BZ of the surface reconstruction. Finally we need to define a projection $P^i_k$ of an arbitrary plane wave $e^{-ik.r}$ onto the Bloch wave function $\psi_{i,k}(r)$ of the $i$-th electronic band as follows:

$$P^i_k = \langle e^{-ik.r}|\psi_{i,k}(r)\rangle = \sum_\nu a^i_\nu(k)\langle e^{ik.(r-R_\nu)}\chi_\nu(r)\rangle \approx \sum_\nu a^i_\nu(k). \tag{5}$$

The approximation above is good if the basis function $\chi_\nu(r)$ are strongly localized around an atom nucleus at $R_\nu$ and the wavelength of light, $2\pi/k$, is much longer than spread of the basis function.

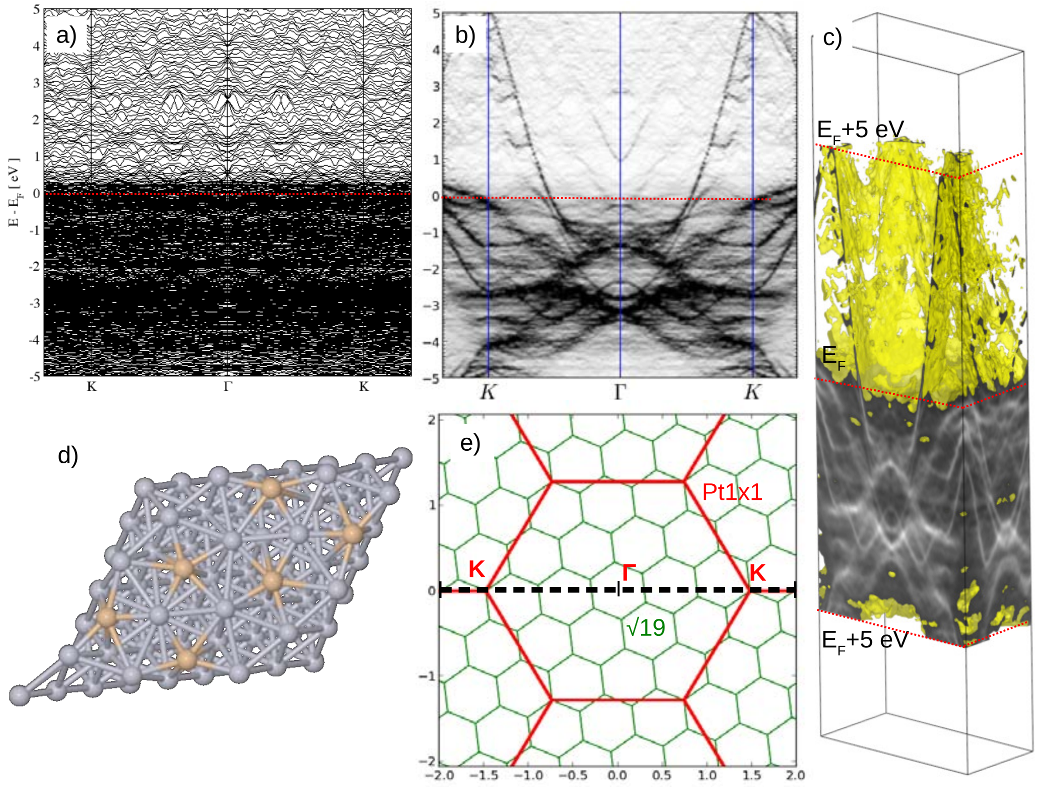


FIG. 13. Unfolding band structure of the $\sqrt{19}$. a) Normal (folded) band structure obtained from eigenvalues of DFT calculation in direction $K\Gamma K$ of Pt(111)-$(1 \times 1)$ of the 1.BZ; b) band structure at the same energy and $k$-vector range as in (a) but unfolded by the projection method described in the text. The folded bands are filtered out by the projection; c) 3D view of the unfolded band structure in the same range; d) geometry of the $\sqrt{19}$ unit cell of the SiPt reconstruction; e) scheme of the reciprocal lattice of the $\sqrt{19}$ (green) and the Pt(111)-$(1 \times 1)$ (red) periodicities. The black line denotes the direction of the slice shown in (a) and (b) respectively.

In practice, we map the 3D space consisting of a discretized energy range and a finite set of $k$-vectors, which cover the reciprocal space of our interest, i.e. the 1. BZ of the clean Pt(111)-1x1 surface. Next, we calculate $P_k^i$ for all the bands located in a given pixel of the 3D energy-momentum space (see Fig.13). The slices of the 3D band structure of the SiPt surface alloy consist of colored pixels representing a sum of all the $|P_k^i|$ of all states within the corresponding energy range.

* corresponding author: svec@fzu.cz

[1] J. Berger, M. Svec, M. Muller, M. Ledinsky, A. Fejfar, P. Jelinek, and Z. Majzik, Beilstein J. Nanotechnol. **25**, 225301 (2013).

[2] J. Lewis, P. Jelínek, J. Ortega, A. Demkov, D. Trabada, B. Haycock, H. Wang, G. Adams, J. Tomfohr, E. Abad, H. Wang, and D. Drabold, Phys. Stat. Sol. B **248**, 1989 (2011).

[3] P. Jelinek, H. Wang, J. Lewis, O. F. Sankey, and J. Ortega, Phys. Rev. B **71**, 235101 (2005).

[4] G. Kresse and J. Hafner, Phys. Rev. B **47**, 558 (1993).

[5] G. Kresse and J. Hafner, Phys. Rev. B **49**, 14251 (1994).

[6] G. Kresse and J. Furthmüller, Comput. Mat. Sci. **6**, 15 (1996).

[7] G. Kresse and J. Furthmüller, Phys. Rev. B **54**, 11169 (1996).

[8] D. Vanderbilt, Phys. Rev. B **41**, 7892 (1990).

[9] G. Kresse and J. Hafner, J. Phys.: Condens. Matter **6**, 8245 (1994).

[10] J. P. Perdew, J. A. Chevary, S. H. Vosko, K. Jackson, M. Pederson, D. Singh, and C. Fiolhais, Phys. Rev. B **46**, 6671 (1992).

[11] J. P. Perdew, J. A. Chevary, S. H. Vosko, K. Jackson, M. Pederson, D. Singh, and C. Fiolhais, Phys. Rev. B **48**, 4978 (1993).

[12] L. Meng, Y. Wang, L. Zhang, S. Du, R. Wu, L. Li, Y. Zhang, H. Z. G. Li, W. A. Hofer, and H.-J. Gao, Nano Lett. **13**, 685 (2013).

[13] J. M. Blanco, F. Flores, and R. Pérez, Prog. Surf. Sci. **81**, 403 (2006).

[14] J. B. Pendry, J. Phys. C **13**, 937 (1980).

[15] G. Held and W. Brown, "Cleed manual. available from the authors,".

[16] J. P. Perdew, K. Burke, and M. Ernzerhof, Phys. Rev. Lett. **77**, 3685 (1996).

[17] E. Wimmer, H. Krakauer, M. Weinert, and A. J. Freeman, Phys. Rev. B **24**, 864 (1981).

[18] M. Weinert, E. Wimmer, and A. J. Freeman, Phys. Rev. B **26**, 4571 (1982).

[19] H. J. Monkhorst and J. D. Pack, Phys. Rev. B **13**, 5188 (1976).

[20] N. Materer, U. Starke, A. Barbieri, R. Döll, K. Heinz, M. A. Van Hove, and G. A. Somorjai, Surf. Sci. **325**, 207 (1995).
